# Supplementary material for: Transforming Podcast Preview Generation: From Expert Models to LLM-Based Systems
Source: arXiv:2505.23908 source file (2025-06-03)
Supplement: Supplementary file 1 [file appendix_preview_comparison.tex]

\section{Comparing Examples of a Legacy ML preview with an LLM preview}
\label{sec:preview_comparison}

\begin{table}[htbp]
\centering
\resizebox{0.8\linewidth}{!}{
    \begin{tabularx}{\linewidth}{X}
    \toprule
    \textbf{Episode Name} \\
    \midrule[0.3pt]
    Lucid Dreaming: The Bonkers World Inside Our Minds \\
    \toprule
    \textbf{Episode Description} \\
    \midrule[0.3pt]
    Some people can control their dreams. While they're fast asleep: they fly, create new worlds, live other lives... \\
    \toprule
    \textbf{Legacy ML Preview} \\
    \midrule[0.3pt]
    So then she recruits 22 folks who couldn't lucid dream and also didn't have narcolepsy, and she repeats the experiment. It's crazy, but they were also able to do the task. So they were indeed asleep according to their brain activity, but they were able to respond. Wait, they could. So we could. So if I went to sleep now and you started asking me what's a word, pizza or pizza, chances are I would respond. It's like there. Are chances It's not all the time, but it looks like there are some transient windows of opening... \\
    \toprule
    \textbf{LLM preview} \\
    \midrule[0.3pt]
    And he gets really into this thing called reality testing or reality checks. And these are huge in the lucid dreaming world. I mean, just ask Christopher Nolan about it. It was an inception. So to understand how this could work, it's helpful to know that often people will spontaneously have a lucid dream because they'll be stuck in the middle of a dream and something really weird will happen that makes them think what this has to be a dream, and voila, they're lucid. And so reality testing is all about trying to hack that process... \\
    \bottomrule
    \end{tabularx}}
      \caption{\label{comparison_example_ml_llm}
        Comparing a legacy ML preview with an LLM preview for the same episode.
      }
\end{table}
% spotify:episode:7KI6uxfrUgYvtancAXc4mf

In Table \ref{comparison_example_ml_llm}, we compare the legacy ML preview and LLM preview for an episode titled ``Lucid Dreaming: The Bonkers World Inside Our Minds.'' The LLM preview begins at the start of a coherent thought and introduces a new concept, serving as an engaging entry point to the full episode. In contrast, the legacy ML preview is a continuation of a previous discussion that lacks context, making it difficult to follow. Empirical evidence suggests that a lack of context or clarity in the first few seconds can significantly influence a user's decision to either skip or engage with a preview. In this instance, the LLM preview proves superior.
