# Supplementary material for: Transforming Podcast Preview Generation: From Expert Models to LLM-Based Systems
Source: arXiv:2505.23908 source file (2025-06-03)
Supplement: Supplementary file 2 [file appendix_preview_metadata.tex]

\section{Preview Metadata Generated through Structured Reasoning Process: Title, Explanation and Topic Tags}
\label{sec:preview_metadata}

Below is an example of preview metadata generated by the LLM for an episode titled ``Lucid Dreaming: The Bonkers World Inside Our Minds.'' The metadata was produced during the structured reasoning process to ensure that the selected preview remains relevant to the episode's theme:

\begin{quote}
\textbf{Episode Theme:} Unlocking Lucid Dreaming: Methods, Science, and Benefits

\textbf{Preview Title:} Does Reality Testing Work?

\textbf{Preview Explanation:} Learn how Australian psychologist Dr. Denham Adventure-Heart uses ``reality testing'' to induce lucid dreaming and the surprising results of his 350-person study.

\textbf{Preview Hash Tags:} \#LucidDreamingHacks, \#RealityTestingDreams, \#DreamScience
\end{quote}
