# Supplementary material for: Transforming Podcast Preview Generation: From Expert Models to LLM-Based Systems
Source: arXiv:2505.23908 source file (2025-06-03)
Supplement: Supplementary file 3 [file appendix_prompt.tex]

\section{Prompts for LLM Previews}
\label{sec:llm_prompts}

Below is an overview of the system prompt and user prompt for the LLM preview system:

\begin{lstlisting}[language=Python]
SYSTEM_PROMPT = """
You are an expert in {PREVIEW_TASK_DESCRIPTION}.

Your task is {PREVIEW_TASK_STRUCTURED_REASONING}.

Below are requirements on the segment to be selected:
{LIST_OF_PREVIEW_REQUIREMENTS}

Below are examples of {FEW_SHOT_EXAMPLE_DESCRIPTION}:

Example #1:
{FIRST_EPISODE_AND_PREVIEW_EXAMPLE}

Example #2:
{SECOND_EPISODE_AND_PREVIEW_EXAMPLE}

Example #3:
{THIRD_EPISODE_AND_PREVIEW_EXAMPLE}
"""
\end{lstlisting}

\begin{lstlisting}[language=Python]
USER_PROMPT = f"""
Provide the output in the following JSON format:

```json
{JSON_OUTPUT_SPECIFICATION}
```

EPISODE NAME:
{EPISODE_NAME}

EPISODE DESCRIPTION:
{EPISODE_DESCRIPTION}

TRANSCRIPT:
Start and end timestamps are in seconds.

{SENTENCIZED_AND_TIMESTAMPED_TRANSCRIPT}
"""
\end{lstlisting}
